# Supplementary material for: High-temperature charge density wave correlations in La$_{1.875}$Ba$_{0.125}$CuO$_{4}$ without spin-charge locking
Source: arXiv:1701.00022 ancillary file (2017-11-22)
Supplement: Supplementary file 1 [file supp.pdf]

# Supporting Information for High-temperature charge density wave correlations in $La_{1.875}Ba_{0.125}CuO_4$ without spin-charge locking

H. Miao,[1,*] J. Lorenzana,[2] G. Seibold,[3] Y.Y. Peng,[4,5] A. Amorese,[6] F. Yakhou-Harris,[6] K. Kummer,[6] N. B. Brookes,[6] R. M. Konik,[1] V. Thampy,[1] G.D. Gu,[1] G. Ghiringhelli,[4,7] L. Braicovich,[4,7] and M. P. M. Dean[1,†]

[1] *Condensed Matter Physics and Materials Science Department, Brookhaven National Laboratory, Upton, New York 11973, USA*

[2] *Istituto dei Sistemi Complessi-Consiglio Nazionale delle Ricerche, Dipartimento di Fisica, Università di Roma "La Sapienza", P. Aldo Moro 2, 00185 Roma, Italy*

[3] *Institut für Physik, Brandenburgische Technische Universität Cottbus-Senftenberg, P.O. Box 101344, 03013 Cottbus, Germany*

[4] *Dipartimento di Fisica, Politecnico di Milano, 20133 Milano, Italy*

[5] *Consiglio Nazionale delle Ricerche-SPIN at Politecnico di Milano, 20133 Milano, Italy*

[6] *European Synchrotron Radiation Facility (ESRF), BP 220, F-38043 Grenoble Cedex, France*

[7] *CNR-SPIN at Politecnico di Milano, 20133 Milano, Italy*

(Dated: November 22, 2017)

## CONTENTS

1. RIXS experimental geommetry (Fig. S1)
2. Self-absorption (Fig. S2)
3. Temperature dependent RIXS intensity map (Fig. S3)
4. Energy-width of the quasi-elastic line at $\mathbf{Q}_{\mathrm{CDW}}$ (Fig. S4)
5. Curve fitting I: CDW (Fig. S5 and S6)
6. Curve fitting II: Magnon (Fig. S7)
7. Paramagnon softening in the stripe ordered CDW phase (Fig. S8 and S9)

## 1. RIXS EXPERIMENTAL GEOMMETRY

In this work, we use similar experimental geometries to those employed previously to study charge and spin scattering (11). Figure S1A shows a top-down view of the scattering geometry. $2\theta$ is the angle between incident and outgoing photon directions and $\boldsymbol{a}^*$ and $\boldsymbol{c}^*$ are the reciprocal lattice vectors. In our measurements, the $2\theta$ value is chosen to be 118° for the CDW such that $L \approx 1.5$ and the CDW structure factor is enhanced. For magnetic excitations we use the maximum available $2\theta = 149°$ in order to access large $H$. In the setup used it was impractical to move the 12 m scattering every point in the scan, so data were taken by rotating the sample only in order to change $H$ the projection of the total $\boldsymbol{Q}$ along $\boldsymbol{a}^*$. In our notation, positive (negative) $H$ corresponds to the grazing exit (grazing incidence) side of the specular condition w.r.t. the $c$-axis surface normal.

The polarization dependent RIXS scattering amplitude can be computed from the Kramers-Heisenberg expression:

$$A_{fi} = \sum_n \frac{\langle f|\,\hat{D}\,|n\rangle \langle n|\,\hat{D}\,|i\rangle}{\hbar\omega - E_n + i\Gamma/2}, \tag{1}$$

where $A_{fi}$ is the scattering amplitude from initial state $i$ to final state $f$. $\hat{D}$ is the polarization dependent dipole operator. $|n\rangle$ is the intermediate state with energy $E_n$, which we assume is much larger than the RIXS energy loss $[E_n \gg (\hbar\omega - \hbar\omega')]$. $\Gamma$ is the core-hole lifetime.

At the Cu $L$-edge, the RIXS process can be written as $2p^4_{3/2}3d^9 \to p^3_{3/2}3d^{10} \to p^4_{3/2}3d^{9*}$, where $*$ indicates that the final states can be either the ground state (i.e. an elastic scattering process) or an excited state. Using a single-site approximation for the resonant process the RIXS intensity ratio between the $\pi$ and $\sigma$ incident x-ray polarization in the charge and spin channel are

$$\frac{I_\pi^{\text{charge}}}{I_\sigma^{\text{charge}}} = \frac{\left[4\sin^2(\delta-\theta) + \cos^2\theta_s\right]\sin^2(\delta+\theta)}{4 + \cos^2(\theta_s)\sin^2(\delta-\theta)} \tag{2}$$

$$\frac{I_\pi^{\text{spin}}}{I_\sigma^{\text{spin}}} = \frac{\sin^2(\delta+\theta)}{\sin^2(\delta-\theta)} \tag{3}$$

where $\theta$ is half of the scattering angle $2\theta$. $\theta_s$ is the angle between spin direction and the sample $c$-axis (which is approximated as 90° following the values for undoped cuprates).

Using Eqs. (2) and (3), we plot the normalized RIXS signal intensities with $\pi$ and $\sigma$ incident polarizations at $2\theta$=118° and $2\theta$=150° in Fig. S1B-E. With $\pi$ polarization and positive $H$, the scattering is dominated by the magnon as seen experimentally. Under $\sigma$ polarization, the charge scattering is stronger. In this case the presence of spin flip excitations contribute to the background in nominally elastic scattering experiments, much of this signal is suppressed in RIXS experiments by energy-resolving the scattered beam.

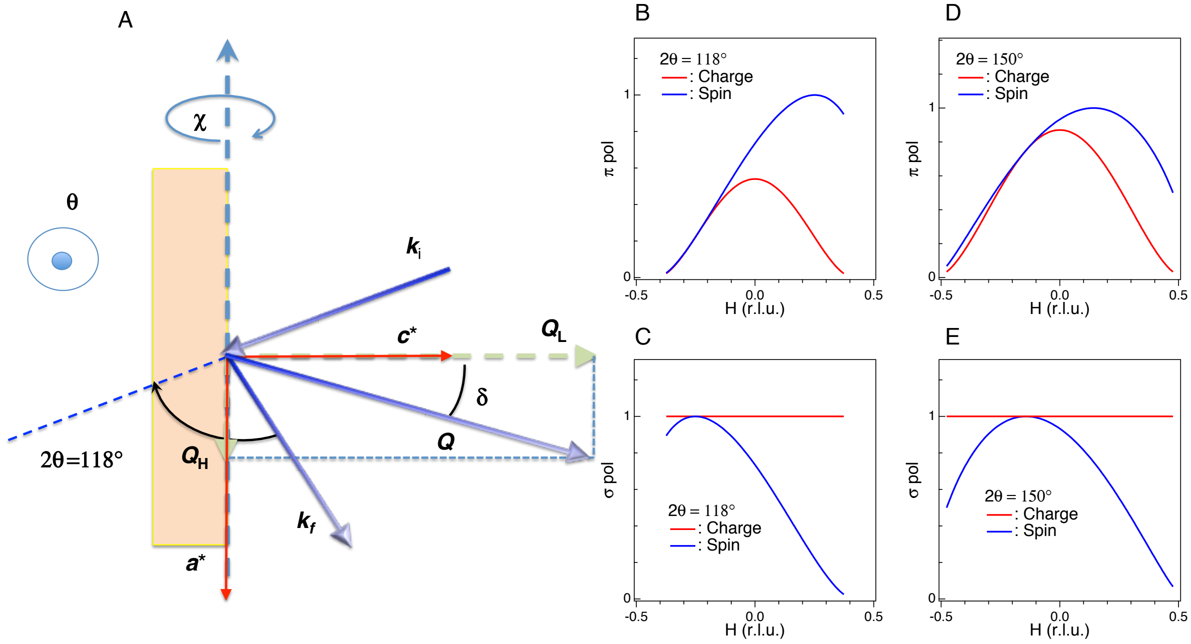


Figure S1. **A**, Top view of the scattering geometry. **B** and **C** are the calculated RIXS scattering intensity at $2\theta = 118°$ with $\pi$ pol and $\sigma$ pol, respectively. **D** and **E** are the calculated RIXS scattering intensity at $2\theta = 150°$ with $\pi$ pol and $\sigma$ pol, respectively.

## 2. SELF-ABSORPTION

In this section we describe x-ray self-absorption effects and how these are accounted for in the data. At the Cu $L_3$ edge, the X-ray attenuation length ($\sim 0.15$ $\mu$m) is much smaller than the sample thickness ($\sim 2$ mm). Hence, the effect of self-absorption can be simplified as

$$\frac{I}{I_0} = \frac{\sin\theta_o}{\sin\theta_i + \sin\theta_o} \tag{4}$$

where $I$ and $I_0$ are scattering intensities with and without self-absorption and $\theta_i$ and $\theta_o$ are the angles of incidence and exit w.r.t. the sample surface. Although a more sophisticated model would consider the photon polarization, that effect is small and can be neglected. We tested this by calculating the off resonant intensity measured in the geometry used for the CDW measurements which is expected to be constant apart from self-absorption effects. Fig. S2 shows that Eq. 4 nicely captures the overall trend observed. Fig. S2B shows the same calculation for the scattering angles used for the magnetic excitations ($2\theta = 149°$). The intensity maps shown in Fig. 4 of the main text are self-absorption corrected using the curve shown in Fig. S2B as the self absorption effect is significant over the measured momentum range.

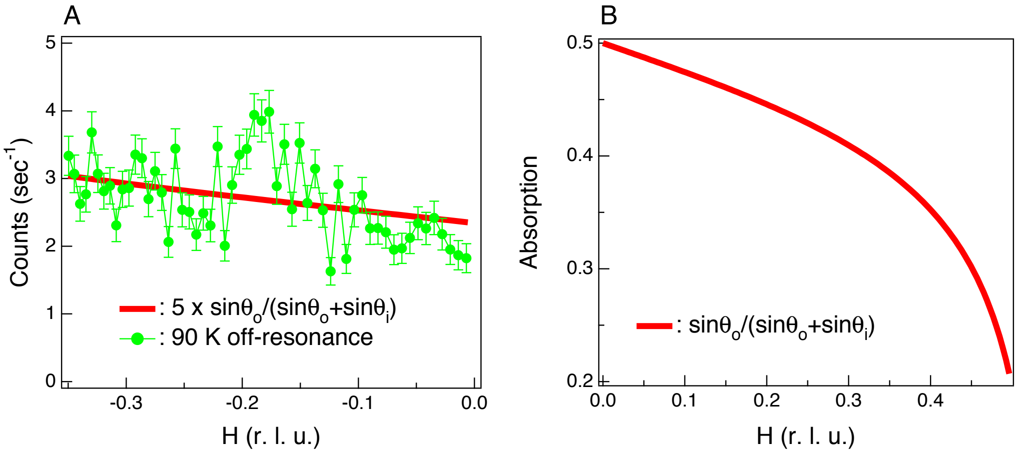


Figure S2. **A**, The calculated self absorption coefficient in the charge scattering geometry (red solid line), which matches the quasi-elastic intensity in the off-resonant condition (green circles). **B**, Simulated self-absorption curve for the magnon measurement.

## 3. TEMPERATURE DEPENDENT RIXS INTENSITY MAPS

For the sake of completeness, we provide the RIXS maps used to construct Fig. 1 in the main text in Fig. S3.

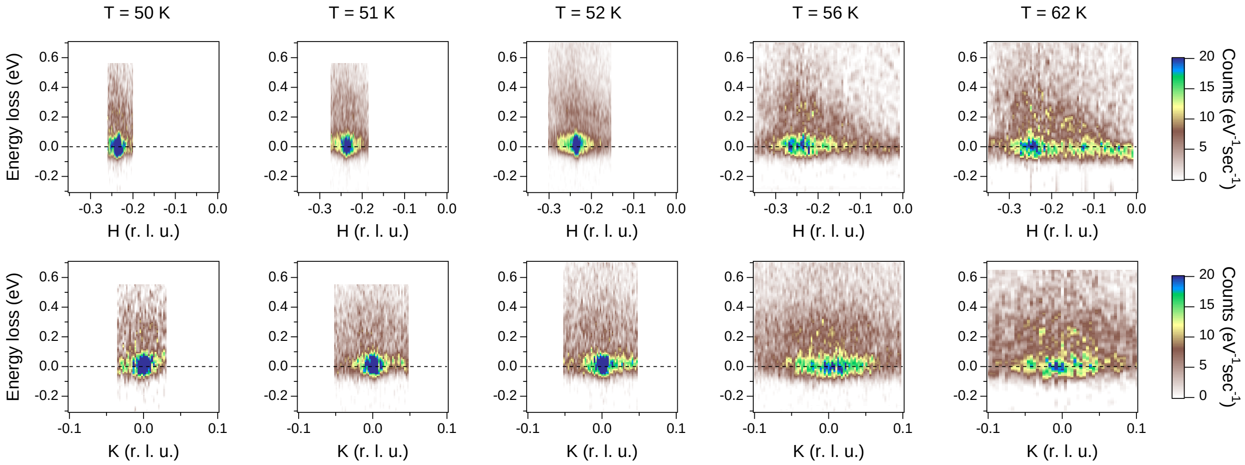


Figure S3. Cu $L_3$-edge RIXS intensity maps above 50 K.

## 4. ENERGY-WIDTH OF THE QUASI-ELASTIC LINE AT $\mathbf{Q}_{\mathrm{CDW}}$

If the high-temperature CDW is dynamic, one would expect an increase in the width of the quasi-elastic line going through the CDW to high-temperature CDW transition. This section shows that such an effect, should it be present, is too small to be resolved here. The temperature dependent RIXS spectra at $\boldsymbol{Q}_{\mathrm{CDW}}$ are shown in Fig. S4. All these spectra are taken from $\chi$-scans and integrated over a momentum window of 0.016 r.l.u. around $\boldsymbol{Q}_{\mathrm{CDW}}$. The quasi-elastic peak is found to be energy-resolution-limited ($\sim$ 90 meV) through all temperatures, indicating fluctuations, if present, are slower than $\tau \sim 100$ fs. A direct comparison of the RIXS spectra below and above the LTT-LTO transition is shown in Fig. S4B. The green and yellow curves are 54 K and 59 K spectra, respectively. The drop of quasi-elastic peak intensity at 59 K in the RIXS spectra corresponds to the disappearance of low temperature CDW above 55 K in the momentum dependent plot of Fig. 1 in the main text.

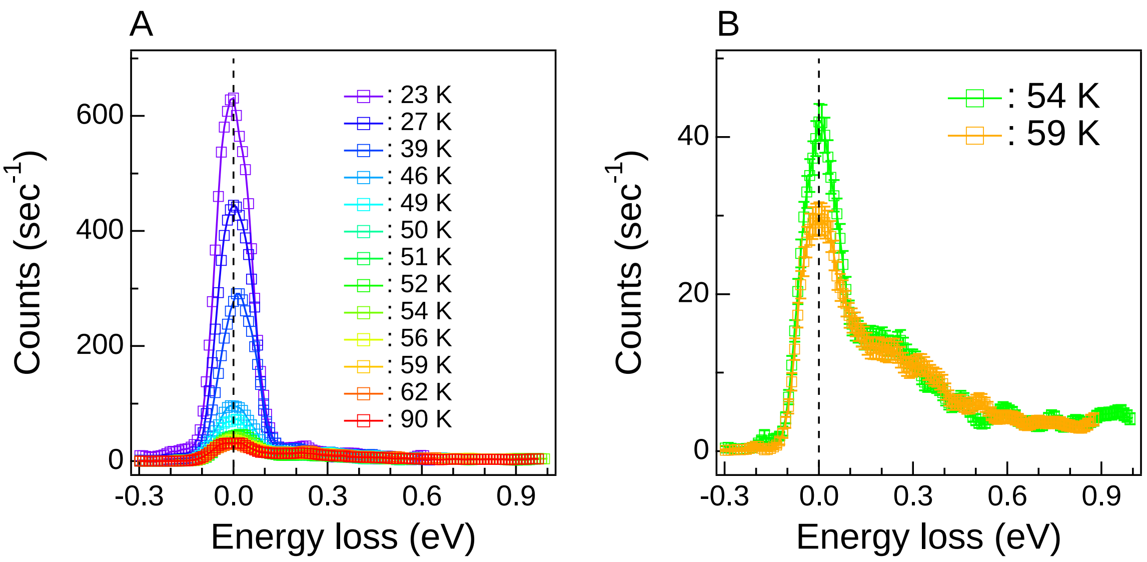


Figure S4. **A**, Temperature dependent RIXS spectra at $\mathbf{Q}_{CDW}$. A comparison of spectra just below (54 K) and above (59 K) the LTT-LTO transition is shown in **B**. The error bars come from Poisson counting statistics.

## 5. CURVE FITTING I: CDW

Here we present the fitting of the RIXS momentum scans integrated in an energy window of ±150 meV around 0 meV. The spectra are fitted by two Lorentzian squared functions plus a linear background:

$$I = c_0 + c_1 * x + P_I^1 \left[ \frac{1}{1 + \left( \frac{x - P_{pos}^1}{P_{wid}^1} \right)^2} \right]^2 + P_I^2 \left[ \frac{1}{1 + \left( \frac{x - P_{pos}^2}{P_{wid}^2} \right)^2} \right]^2, \tag{5}$$

where $P_I$, $P_{pos}$ and $P_{wid}$ represent peak intensity, position and width respectively, and $x$ can be $H$ or $K$. Superscripts differentiate the two peaks $P^1$ and $P^2$, which account for the sharp CDW peak observed at low temperature and the broad high-temperature peak observed most clearly at high temperatures, but also persisting at low temperatures. The linear term $c_0 + c_1 * x$ is used to account for the background. We chose the Lorentzian squared function on a phenomenological basis as it reproduces the observed peak shape better than other functions such as Lorentizian or Gaussian lineshapes. The same function has also been used previously in the literature (17, 29).

We start with fitting the broad high-temperature data (> 55 K), where only the high-temperature CDW peak is observed along both $H$ and $K$ directions. In this case, we set $P_I^2$ to be zero. Representative fitting parameters and fitted curves at 59 K and 90 K are shown in Fig. S5. The peak width and intensity shown in Fig. 3 in the main text were calculated by taking the mean of the fitting parameters obtained from the $H$ and $K$ scan fits. The error bars were determined by the larger standard error of the fitting parameters.

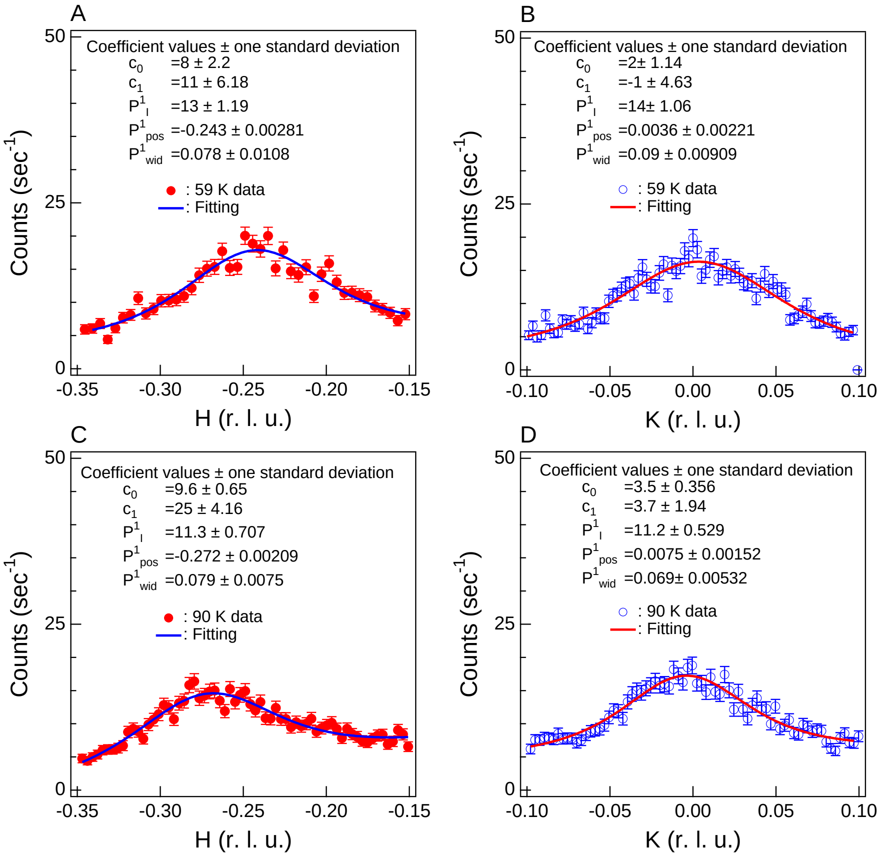


Figure S5. A demonstration that the high-temperature CDW peak can be modeled accurately by fitting a Lorentizian squared function. The fitting curve and fitting parameters are shown in each panel. **A** and **B** plot cuts along $H$ and $K$ respectively at 59 K and **C** and **D** show the same data at 90 K, which also demonstrates a clear shift towards larger absolute $H$.

The low temperature intensity has three contributions: Low temperature CDW, high-temperature CDW and a linear background. As shown in Fig. S6 A and E, within experimental uncertainties, the shape of the broad intensity (that including both high-temperature CDW peak and linear background) is constant below 62 K. This allows us to fix the fitting

parameters of the broad high-temperature CDW and linear background in Eq. 5. Representative fitting results of the low temperature spectra along $H$ and $K$ directions are shown in Fig. S6 (B-D) and Fig. S6 (F-H), respectively. Here the fixed parameters for the linear background and the high-temperature CDW are taken from the 59 K data.

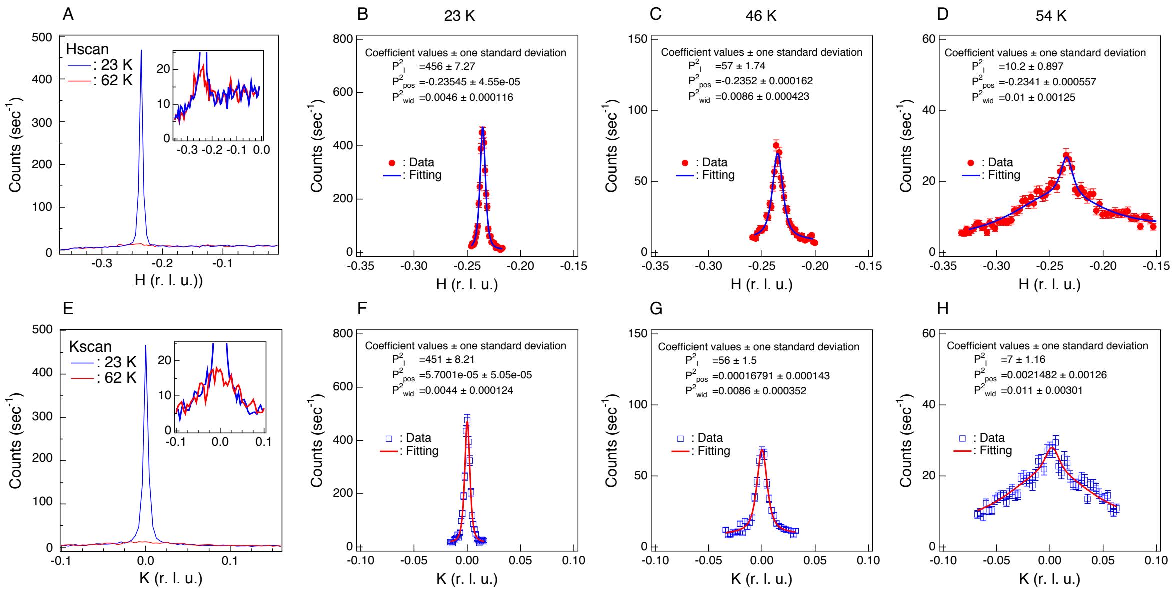


Figure S6. **A**,**E** Comparison of the low-temperature (23 K) and high-temperature (62 K) RIXS intensity along $H$ and $K$, respectively, shown over wide ranges of reciprocal space. The inset panels show the same data but with smaller vertical scales. Integrated RIXS intensity and the fitting at 23 K, 46 K and 54 K along $H$ (**B-D**) and $K$ (**F-H**) directions are shown in the other panels.

## 6. CURVE FITTING II: MAGNON

The total RIXS spectrum is the sum of three functions, which account for the quasi-elastic scattering, magnon (or paramagnon if $T > T_{SDW}$), and background which comes from charge transfer excitations and the tail of the dd-excitations, respectively (53). A Gaussian function of FWHM 70 meV, which is a good approximation to the instrumental resolution function, was used to fit to the quasi-elastic peak. An antisymmetrized Lorentzian was fit to the (para)magnon, and a linear function to the background. The scattering intensity $S(\mathbf{Q}, \omega)$ depends on the imaginary part of the dynamical susceptibility $\chi''(\mathbf{Q}, \omega)$ and the sample

temperature $T$:

$$S(\mathbf{Q},\omega) \propto \frac{\chi''(\mathbf{Q},\omega)}{1-e^{-\hbar\omega/k_BT}} \tag{6}$$

where $k_B$ and $\hbar$ are the Boltzmann constant and the reduced Planck constant. Due to time reversal symmetry, the dynamical susceptibility must be an odd function of $\omega$, and we model this with an antisymmetrized Lorentzian as:

$$\chi''(\mathbf{Q},\omega) = \frac{\Gamma_{\mathbf{Q}}}{(\hbar\omega-\hbar\omega_{\mathbf{Q}})^2+\Gamma_{\mathbf{Q}}^2} - \frac{\Gamma_{\mathbf{Q}}}{(\hbar\omega+\hbar\omega_{\mathbf{Q}})^2+\Gamma_{\mathbf{Q}}^2} \tag{7}$$

where $\Gamma_{\mathbf{Q}}$ and $\omega_{\mathbf{Q}}$ are scattering rate and pole energy at momentum $\mathbf{Q}$. This form for $S(\mathbf{Q},\omega)$ was convolved numerically with the Gaussian resolution function.

Figure S7A to S7C are RIXS spectra at $\boldsymbol{Q}$=0.2, 0.25 and 0.3 r.l.u., respectively. Purple and red curves are spectra at 23 K and 60 K, respectively. The zero energy loss is determined by the non-resonant elastic scattering spectrum of carbon tape, which is measured before and after each RIXS spectrum. It is evident in the raw data, that at $\boldsymbol{Q}$=0.2, 0.25 and 0.3 r.l.u., an obvious magnon peak shift and spectral weight transfer can be observed. Figures S7D-I show the fits to the spectra shown in Fig. S7A-C. The grey, orange and cyan dashed curves are the linear background, quasi-elastic peak and (para)magnon, respectively. The blue solid curves are the total fit to the raw data shown with open circles. The fitted magnon peak positions are summarized in Fig. 4 of the main text and show a clear magnon softening at low temperatures.

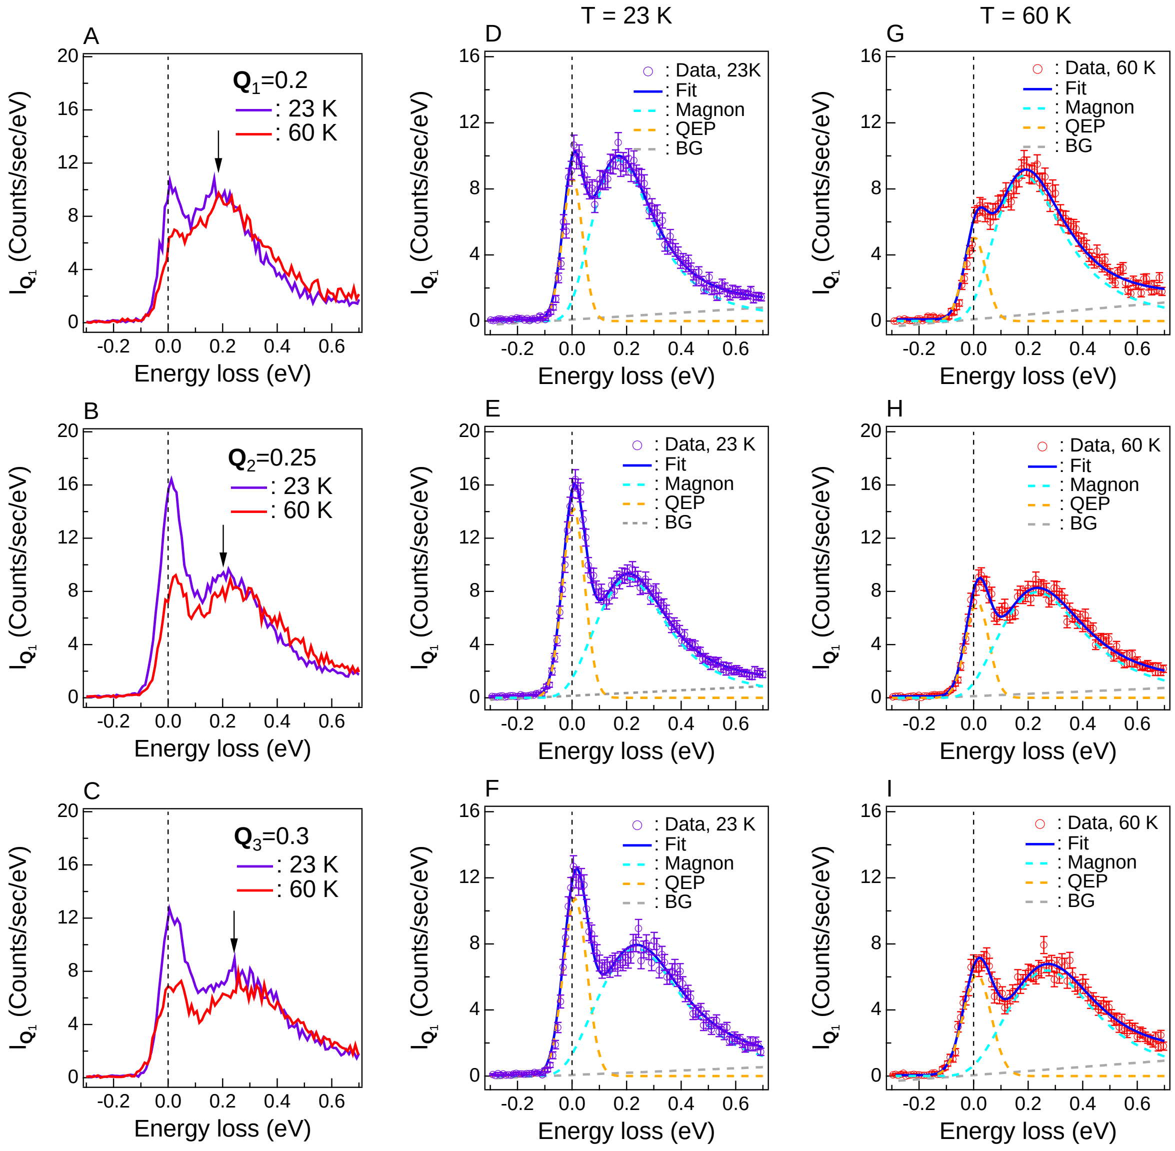


Figure S7. **A**, **B** and **C** RIXS spectra at $\boldsymbol{Q}$=0.2, 0.25 and 0.3 r.l.u., respectively. Black arrows indicate the magnon peak position at low temperature. An obvious peak shift and spectral weight transfer is visible at $\boldsymbol{Q}$=0.25 and 0.3 r.l.u., proving magnon softening at these vectors. **D-F** and **G-I** are fits to the low temperature and high temperature data respectively.

## 7. PARAMAGNON SOFTENING IN THE STRIPE ORDERED CDW PHASE

In this section we present additional calculations of the magnetic excitation spectrum and how it relates to the CDW. The simplest approach is to use a Heisenberg model that only accounts for the spin degree of freedom (53-55), neglecting charge dynamics. It is assumed

that all Cu sites host a spin moment, that are coupled by the magnetic exchange constant $J$. The spin wave theory (SWT) for such a simple model yields a magnon energy dispersion in the absence of doped holes:

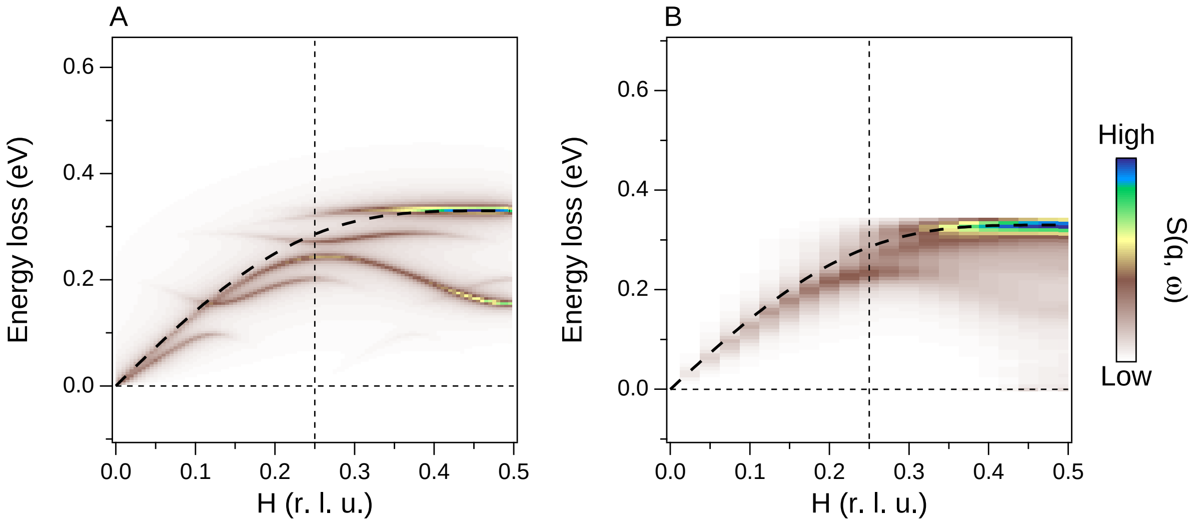


Figure S8. The predicted magnetic excitation spectrum for the fully stripe-ordered state (**A**) and with meandering quasi-ordered stripes (**B**). The magnon energy predicted in the antiferromagnetic phase (Eq. 8) is plotted as a black dotted line.

$$\hbar\omega = 2J\sqrt{1 - \frac{(\cos k_x + \cos k_y)^2}{4}}. \tag{8}$$

As explained in the main text, one can try to capture the effect of the stripe ordered CDW by assuming that doped holes define domain walls on top of an otherwise perfectly AF ordered state and that each site with a hole has a locally modified magnetic exchange interaction changing $J \to J_F$.

We first assumed a fully ordered state where the CDW consists of vertical domain walls every four lattice units. This was the conceptual picture presented by Tranquada et al. as a means of explaining the positions of the charge and magnetic Bragg peaks (9). The magnetic dynamical structure factor, $S(q,\omega)$, of this model can be straightforwardly computed under the spin wave theory approximation. Figure S8A plots the results having averaged over the two possible orientations of stripe domains. The magnetic exchange constants in the model were $J$ = 165 meV and $J_F = -0.09J$ which were fixed from several consistent measurements as described in the main text. As expected, such a model predicts Goldstone

modes that define the magnetic Bragg peaks consistent with those seen by neutron scattering (9, 47). However, comparing with the experimental data shown in Fig. 4 of the main manuscript, the prediction shows several (para)magnon branches with large spectral weight. Most notably, an additional unobserved branch, coming from modes that propagate along the charge stripe, appears at high $H$ at approximately half the energy of the (para)magnon. A more sophisticated modeling of a similar ordered stripe state, as presented in Ref. (57), yields less weight in this extra branch but extra modes still in disagreement with experiment.

As we describe in the main manuscript, the low temperature CDW condenses only a small fraction of the available low energy correlations and appears to be embedded alongside very short range CDW correlations. This motivated us to calculate the magnetic excitation spectrum of electronic configurations that reproduce the experimentally observed charge correlation. In the initial starting configuration, stripes were spaced by 4 lattice units in order to reproduce the observed wavevector and we assume that the stripes have a width of two lattice units where the hole concentration is higher. Note that had we assumed a stripe with a width of one lattice unit, this would predict appreciable $2\boldsymbol{Q}_{\mathrm{CDW}}$ satellite peak intensity that we do not observe here. The disordered states were generated by a Metropolis Monte Carlo algorithm with a fictitious temperature where the energy in the conventional Metropolis algorithm was replaced by the mean-square error between the structure factor of the charge configuration at a given Monte Carlo step and a target structure factor. The latter was chosen to reproduce the main characteristics of the experimental charge structure factor. Charges were moved in horizontal pairs in such a way that vertical stripes keep continuity and do not overlap as explained in the Methods section of the main article. We use a fictitious temperature such that moves that increase the mean-square error are very rare (less than 1%). Typically after 40000 Monte Carlo steps the error saturates at a minimum value and the algorithm stops. It is assumed that the charge stripes define domain walls across which magnetic exchange $J$ is replaced by a ferromagnetic exchange $J_F$. $J = 165$ meV was chosen to match our observed zone boundary magnon energy and $J_F = -0.09J$ was chosen to obtain the correct energy for the neck of the hourglass in Ref. (69). In the case of a meandering stripe, we insert an additional $J_F$ parallel to the stripe direction, in order to maintain well defined, unfrustrated domain walls in the colinear AF order.

Fig. S9A,D shows disordered stripe configurations which reproduce the charge structure factor of the experiment. Each orange/dark-red site is a hole rich site representing around

1/4 of a doped hole with up/down spin. There are equal numbers of hole rich sites and hole poor sites (black and white) giving a nominal doping of 1/8 holes per site as in the experiment. Panels b and e show the charge structure factor of the corresponding configuration on the left column and panels c and f compare a horizontal scan of the structure factor with the target model. The first row (a,b,c) corresponds to the high temperature state while the second row (d,e,f) is the low temperature state. The charge configuration corresponding to d is shown as an inset in Fig. 4 of the main article. As the beam-size in the experiment is much larger than the domain size, the theoretical magnetic dynamic structure factor was averaged over the two possible orientations of the domains.

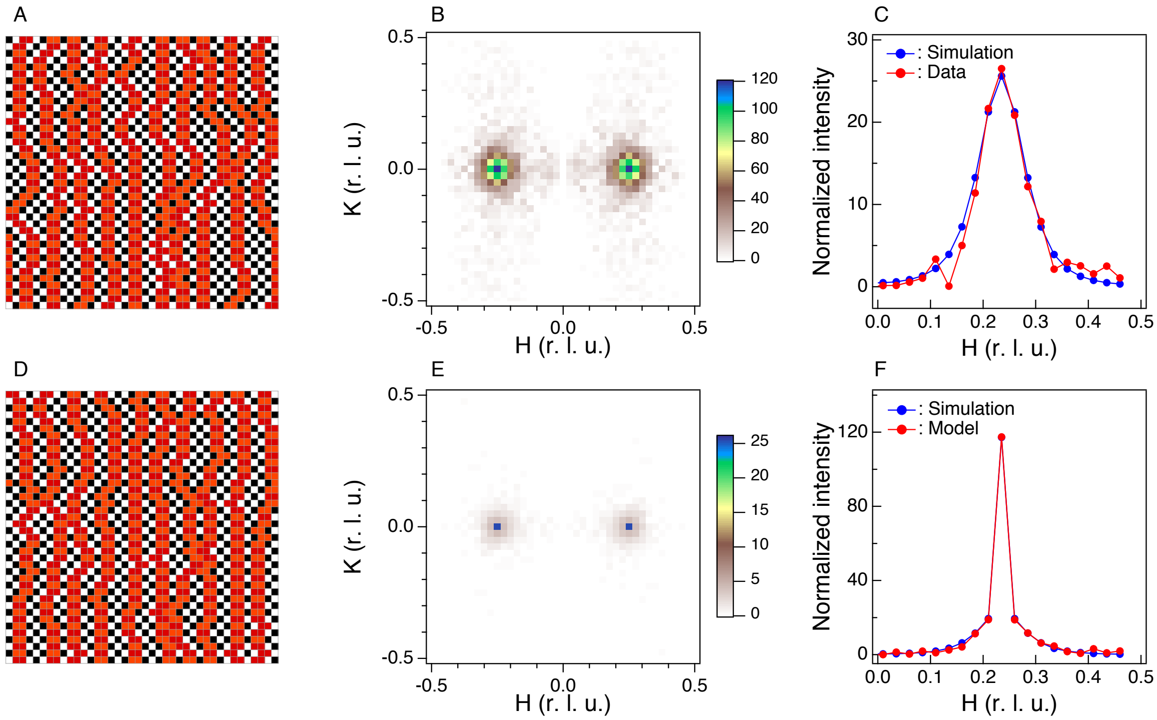


Figure S9. Monte Carlo simulation results for the high temperature charge configuration (**A**, **B**, **C**) and the low temperature charge configuration (**D**, **E**, **F**). **A** and **D** are the final charge and spin configurations. White and black squares represent up and down spins in hole poor sites while orange and red are up and down spins in hole rich sites. The exchange couplings are inserted following the prescription given in the Methods section which results in an unfrustrated collinear magnetic texture (i.e. neighboring sites with the same spin direction are joined by ferromagnetic coupling). **B** and **E** are the corresponding charge structure factors and **C** and **F** compare a cut of the target model with the simulation. The target model is defined by the fitted CDW lineshape in Eq. (5) with parameters similar to the experimental ones. For the high temperature state, Lorentzian squared functions were located at $(H, K) = (\pm\delta, 0)$ with $\delta = 0.25$ r.l.u. The width was set to 0.08 r.l.u. in both $H$ and $K$ directions and the total intensity was fixed by sum rule considerations. For the low temperature state, we sum, at each equivalent point, two Lorentzian squared functions, one with the same parameters as before and the other with the same $\delta$ but with a width of 0.008 r.l.u. The total intensity ratio of the narrow to broad peak functions was set to 1/7, also similar to the experiment. Notice that the narrower peak is resolution limited due to the finite size of the real space lattice ($40 \times 40$) yielding a finite separation of points in momentum space.

Within the adopted model, there is no magnetic frustration and the lowest energy spin configuration is collinear. We also tried another model, allowing the charged stripes to be cut in segments as appears to be the case at very low doping (37). Domain wall formation in such model becomes frustrated since the AF regions become connected. This leads to spin canting, and more importantly, to an unphysical large value of $J_F$, which is needed to obtain a magnetic incommensurability matching the experiment. Furthermore, such large $J_F$ places the neck of the hourglass at too high an energy compared with experiments. This imposes strong constraints on the possible charge configurations that reproduce the present charge correlations that were taken into account in the chosen model with uninterrupted rivers of charge. It is worth mentioning that stripe segmentation probably plays a role on the decoupling of the spin and charge incommensurability observed above 54 K. Indeed, introducing a few cuts shift the magnetic incommensurability in the right direction.

Calculations of the dynamical structure factor are shown in Fig. S8B as well as Fig. 4d of the main manuscript for the low temperature state in which a sharp CDW peak co-exists with the broad diffuse scattering. This yields substantially better agreement with our measurements as compared with a classical stripe crystal (Fig. S8A) and reproduces a similar paramagnon softening to that observed using parameters that are fixed based on other measurements. Upon heating through the transition, the experimental paramagnon softening is reduced consistent with a weakening of the CDW correlations and seemingly independent charge and spin fluctuations. In the theoretical computations, temperature effects where taken into account by choosing an appropriate charge configuration to match the experiment, but were not directly included when applying SWT. We see little difference in our predictions between the low and high temperature states. This might suggest that temperature effects play an important role directly modifying the spin correlations at higher temperatures and not only by modifying the charge configuration.

---

* hmiao@bnl.gov

† mdean@bnl.gov
